# Supplementary material for: Multi-finger Manipulation via Trajectory Optimization with Differentiable Rolling and Geometric Constraints
Source: arXiv:2408.13229 source file (2024-12-10)
Supplement: Supplementary file 1 [file appendix.tex]

\clearpage
% \onecolumn
% \begin{appendices}

\newpage
\appendix
\addcontentsline{toc}{section}{Appendix} % Add the appendix text to the document TOC
\subsection{Trajectory Initialization Details}

The initialization for actions at the first step is sampled from normal distributions with a mean of 0. 
The standard deviation for delta actions $\hat{\mathbf{u}}_t$ is $2.5 \times \mathrm{10}^{-2}$ and for force is between $1.5 \times \mathrm{10}^{-2}$ and $1.5$, which is manually tuned depending on the task and which finger to use.
The initialization for the joint configurations is produced by iteratively adding the delta actions to the previous joint configurations, i.e., $\mathbf{q}_{t+1} = \mathbf{q}_t + \hat{\mathbf{u}}_t$. The standard deviation of the normal distribution for each dimension is tuned according to the task. 
\subsection{Pregrasp}
In our experiments, the robot either begins with grasping the object(e.g., cuboid alignment, cuboid turning, complex reorientation) 
or operates in two distinct manipulation phases (e.g., valve turning and screwdriver turning): 
pregrasping and turning. The distinction depends on whether the robot can remain static without robot contact.
For pregrasping, we slightly modify our trajectory optimization: we remove all the constraints except the contact constraints at the final step. Since pregrasping and choosing contact points are not the scope of this work, we choose the robot's initial pose so that the fingers are very close to the desired contact points. This section mainly focuses on the turning phase. 

\subsection{Additional Constraint for Screwdriver Turning}

Since the precision screwdriver is designed to be used with an index finger pushing the top, we introduce another constraint making sure that the contact between the index finger and the screwdriver only happens at the desired region (top):
$||\mathbf{c}_{0,t} - \hat{\mathbf{c}}(\mathbf{o}_t)|| - h \le 0,$ 
where $\mathbf{c}_{0,t}$ is the contact point between the index finger and the object, $h=2~\text{cm}$, and $\hat{\mathbf{c}}(\mathbf{o}_t)$ is the ideal contact location, which is the center of the top surface of the screwdriver. 

\subsection{Size of the manipulated object}
\textbf{Valve Turning:} The cross-shaped valve consists of two cuboids measuring $2~\text{cm} \times 2~\text{cm} \times 20~\text{cm}$.

\textbf{Screwdriver Turning: }
We model the screwdriver handle as a cylinder with $2~\text{cm}$ radius and $10~\text{cm}$ length, and the shaft as another cylinder with $0.5~\text{cm}$ radius and $10~\text{cm}$ length.  

\textbf{Cuboid Alignment: }The cuboid is a $4~\text{cm} \times 4~\text{cm} \times 30~\text{cm}$.

\textbf{Cuboid Turning: }The cuboid measures $4~\textbf{cm} \times 4~\textbf{cm} \times 10~\textbf{cm}$.

\textbf{Complex Reorientation: }The approximate dimension of the object is $15~\text{cm} \times 4~\text{cm} \times 1~\text{cm}$. 

\subsection{Optimization Iterations}
In both our method and the ablation method, for valve turning, we use 100 for warm-up and 30 for online. For screwdriver turning and cuboid alignment, we use 300 for warm-up and 50 for online. For cuboid turning and complex reorientation, we use 200 for warm-up and 30 for online. 
However, we reduce the online iterations to 10 for real-world experiments to slightly speed up the algorithm.

For MPPI, we use 5 iterations initially to warm up and use only 1 iteration online.
